# Supplementary material for: An Unpaired Shape Transforming Method for Image Translation and Cross-Domain Retrieval
Source: arXiv:1812.02134 source file (2021-08-18)
Supplement: Supplementary file 1 [file 6-supp.tex]

\setcounter{section}{0}
\setcounter{figure}{0}
\setcounter{table}{0}
%To number supplemental material with 'S': 

% \renewcommand{\thefigure}{\Alph{section}\arabic{figure}}
% \renewcommand{\thetable}{\Alph{section}\arabic{table}}
%%====================================

% \section{Supplementary material}
% \vspace{-0.2cm}
% \label{supp}

This supplementary material includes more 
experimental results~(Sec.~\ref{sec:supp_exp}), 
as well as additional implementation details 
regarding the network architecture and training~(Sec.~\ref{sec:supp_implement}) 
of the proposed method.

%%%%%%%%%%%%%%%%%%%%%%%%%%%%%%%%%%%%%%%%%%%%%%%
\section{Additional experimental results}
\label{sec:supp_exp}
In this section, we provide more results for  
clothing translation, face translation and clothing retrieval experiments. 

% \myparagraph{Ablation Study: Clothing try-on / take-off}
\subsection{Ablation Study: Clothing try-on / take-off}
This ablation study experiment follows the same settings as
presented in Sec.~4.1 of the 
submitted manuscript. 
Here, we provide additional results for both the clothing 
try-on task~(Fig.~\ref{fig:Supp_FashionStyle_ABL_tryon}) 
and the clothing try-off task~(Fig.~\ref{fig:Supp_FashionStyle_ABL_takeoff}) 
on our FashionStyle dataset. These are extended versions of Fig.~4 in the main paper.

In addition, we conduct an experiment to highlight 
the effectiveness of the proposed fit-in module 
for both unsupervised and supervised models by removing the context input and the Fit-in module.
% in the context of a supervised model. 
% For this, the supervised model
% For the unsupervised model, we remove the context input and the Fit-in module.
% As to the supervised model, the
% architecture is a residual block based on U-net similar to PG$^2$~\cite{ma2017pose} as described in Sec. 4.1.
% \tinne{Add details on what supervised model you're using.}
We provide the results with and without the proposed Fit-in module, shown in Fig.~\ref{fig:Supp_FashionStyle_super_fitin_p1} and Fig.~\ref{fig:Supp_FashionStyle_super_fitin_p2}. 

We can observe that without the Fit-in module, the generated clothing part loses texture details and the generated/translated images look  unrealistic. These observations seem to be consistent across both the tested supervised and unsupervised methods.
A possible explanation for this behavior could be that it is difficult for the network to generate the whole person when only given the cloth appearance information, since there are multiple possible valid outputs. 
Additional qualitative results on the FashionStyle dataset are provided in Fig.~\ref{fig:Supp_FashionStyle_quality_tryon} and Fig.\ref{fig:Supp_FashionStyle_quality_takeoff} for try-on and take-off tasks, respectively. For results on the VITON dataset, a large size version of Fig.~5 (from the submitted manuscript) is shown in Fig.~\ref{fig:Supp_VITON_quality}.

% \vfill\null
% \columnbreak
% \newpage

% \myparagraph{Clothing retrieval.} 
\subsection{Clothing retrieval.}
The setting of this clothing retrieval experiment was presented in the main paper (Sec.~4.4). Here, we show more results in Fig.~\ref{fig:Supp_retrieval} (similar to Fig.~8 in the main paper).

% \myparagraph{Face shape translation.} 
\subsection{Face shape translation.}
This face shape translation experiment follows the same protocol as that presented in Sec.~4.5 of the submitted manuscript. Here, we show additional results in Fig.~\ref{fig:Supp_face_quality} (similar to Fig.~9 in the main paper).

In addition, in order to verify whether our method is overfitting to a specific example or suffering from mode collapse, we run a Nearest Neighbor analysis where the translated front view is used to query the frontal view images from the training set. The results in Fig. \ref{figure_nn} indicate that our model does not overfit the training set.

\begin{figure}
  \centering
  \includegraphics[width=1.0\linewidth]{supp_imgs/face_nn.pdf}\\
\vspace{-1mm}
  \caption{\footnotesize{The top-5 nearest neighbors from the training data for face.}}
\label{figure_nn}
\vspace{-0mm}
\end{figure}

% \vfill\null
% \columnbreak
% \newpage

\subsection{Failure cases.}
Our method is not perfect. We show some failure cases in Fig.~\ref{figure_failures}. On clothing data, the failures are usually caused by incorrectly estimated masks and heavy occlusion caused by other clothing items.
% and lacking inner-outer semantic information \jose{find better term?}.
For the face translation task, the failures are mainly caused by incorrectly estimated masks, large pose variation, facial hair and inconsistent skin colors.

\subsection{Style code visualization.}
Here we take a deeper look at the style representation learned by our model. We take this look by generating t-SNE visualizations\footnote{https://github.com/ml4a/ml4a-guides/blob/master/notebooks/image-tsne.ipynb} from the 8-dim style code computed from all the images on the test set of the FashionStyle dataset.

% \jose{
% Following the protocol from here~\footnote{https://github.com/ml4a/ml4a-guides/blob/master/notebooks/image-tsne.ipynb} we generate the results.
% }

Fig.~\ref{fig:tsne_ori} and Fig.~\ref{fig:tsne_grid} indicate that the color information is dominating,
while within similar colors, the style code also
captures the patterns, printed-text and logos from the clothing items.

% %%===========================

% %\clearpage
% \begin{table}[t]
% \centering
% % \footnotesize
% % \begin{tabular*}{17cm}
% \begin{tabular}
% {@{\extracolsep{\fill}} l c c c c c c c c c c c c c}
% \toprule 
% Translation &$n_1$ &$n_2$ &$n_3$ & Minibatch & Learning rate & $\lambda_\text{CC}$ & $\lambda_\text{SR}$ & $\lambda_\text{LR}$ & $\lambda_\text{Sym}$ & $\lambda_\text{P}$ & $\lambda$ & Iteration  \\
% \midrule[0.6pt]	
% 	Clothing try-on  &1 &3 &4 &1 &4e-5 &5 &10 &10 &10 & 5  &1e4 &$\sim$60k \\
% 	Clothing take-off &1 &3 &4 &1 &4e-5 &5 &10 &10 &10 & 2.5  &2e4 &$\sim$60k \\
% 	Face try-on &1 &2 &4 &2 &4e-5 &5 &10 &10 &10 &0.075 &6e5 &$\sim$60k \\
% 	Face take-off &1 &2 &4 &2 &4e-5 &5 &10 &10 &10 &0.025 &2e6 &$\sim$60k \\
% \bottomrule[1pt]

% \end{tabular}
% \caption{Network architecture and training parameters details.}
% % \vspace{+100mm}
% \label{tab:param}
% \end{table}

%%===========================

\begin{figure}
  \centering
  \includegraphics[width=1.0\linewidth]{supp_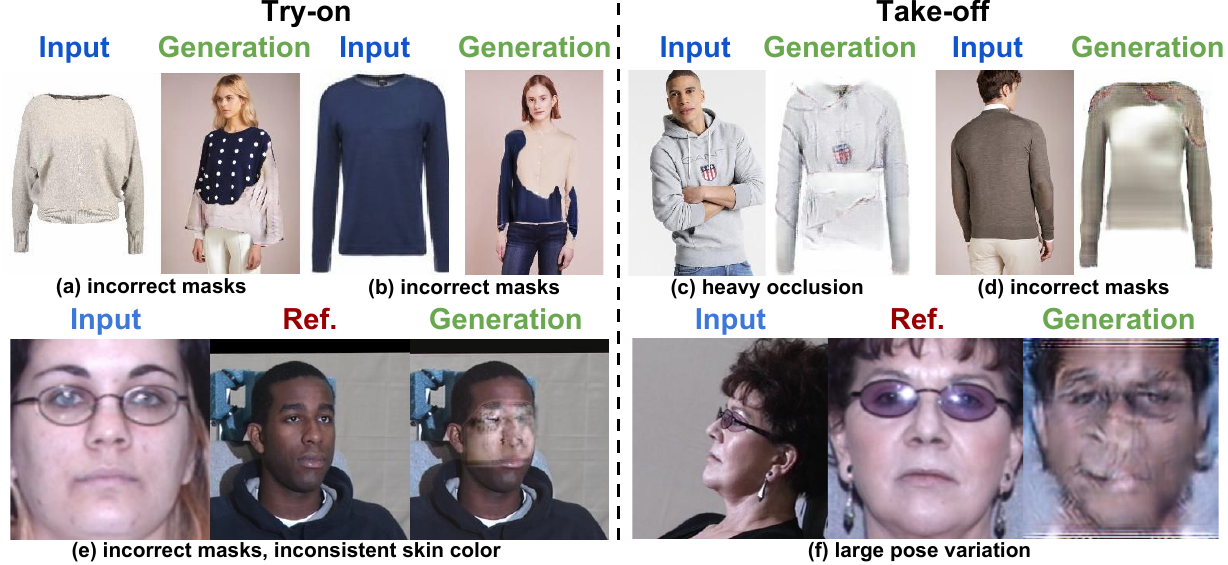}\\
\vspace{-1.5mm}
  \caption{\footnotesize{Failure cases caused by different reasons.}}
\label{figure_failures}
\vspace{-2.5mm}
\end{figure}

%%===========================

%%%%%%%%%%%%%%%%%%%%%%%%%%%%%%%%%%%%%%%%%%%%%%%
\section{Implementation details}
\label{sec:supp_implement}

Table~\ref{tab:param} summarizes the details of 
network architecture presented in  Fig.~3 of the submitted manuscript.
Furthermore, we specify the training parameters used for the tasks analyzed in our experiments.
The number of input/output convolution blocks is set to $n_1=1$. The number of down-sampling and up-sampling convolution blocks is set to $n_2=3$ and $n_2=2$ for clothing and face translation, respectively. We need a different value here, since the images from the two datasets have different resolutions. 
The number of residual blocks is set to $n_3=4$ for both clothing and face translation experiments. As for our Fit-in module, it consists of one
residual block to merge the features with the context information.

% \begin{wraptable}{c}{1\linewidth}
% \centering
% % \footnotesize
% \begin{tabular*}{16cm}
% {@{\extracolsep{\fill}} l c c c c c c c c c c c c}
% \toprule 
% Translation &$n_1$ &$n_2$ &$n_3$ & Minibatch & Learning rate & $\lambda_\text{CC}$ & $\lambda_\text{SR}$ & $\lambda_\text{LR}$ & $\lambda_\text{P}$ & $\lambda_\text{Sym}$ & Iteration  \\
% \midrule[0.6pt]	
% 	Clothing  &1 &4 &4 &1 &2e-5 &10 &10 &10 &10 &10  &$\sim$60k \\
% 	Face &1 &3 &4 &2 &2e-5 &10 &10 &10 &10 &10 &$\sim$60k \\
% \bottomrule[1pt]
% \end{tabular*}
% \caption{Network architecture and training parameters.}
% \vspace{-1mm}
% \label{tab:seg}
% \end{wraptable}

%%%%%%%%%%%%%%%%%%%%%%%%%%%%%%%%%%%%%%%%%%%%%%%
\begin{figure*}[thb]
\centering
\includegraphics[width=0.98\textwidth]{supp_imgs/abl_tryon_supp_v2-crop.pdf}
\caption{
Ablation study on the \textbf{FashionStyle dataset}: \textbf{Try-on task}.
The first two columns show the input clothing product image and the reference ground truth image. The other columns show the generated results for different model settings.}
\label{fig:Supp_FashionStyle_ABL_tryon}
% \vspace{-4mm}
\end{figure*}

\begin{figure*}[thb]
\centering
\includegraphics[width=0.8\textwidth]{supp_imgs/abl_takeoff_supp-crop.pdf}
\caption{
Ablation study on the \textbf{FashionStyle dataset}: \textbf{Take-off task}.
The first two columns show the input clothing product image and the reference ground truth image. The other columns show the generated results for different model settings.}
\label{fig:Supp_FashionStyle_ABL_takeoff}
% \vspace{-4mm}
\end{figure*}

\begin{figure*}[thb]
\centering
\includegraphics[width=0.8\textwidth]{supp_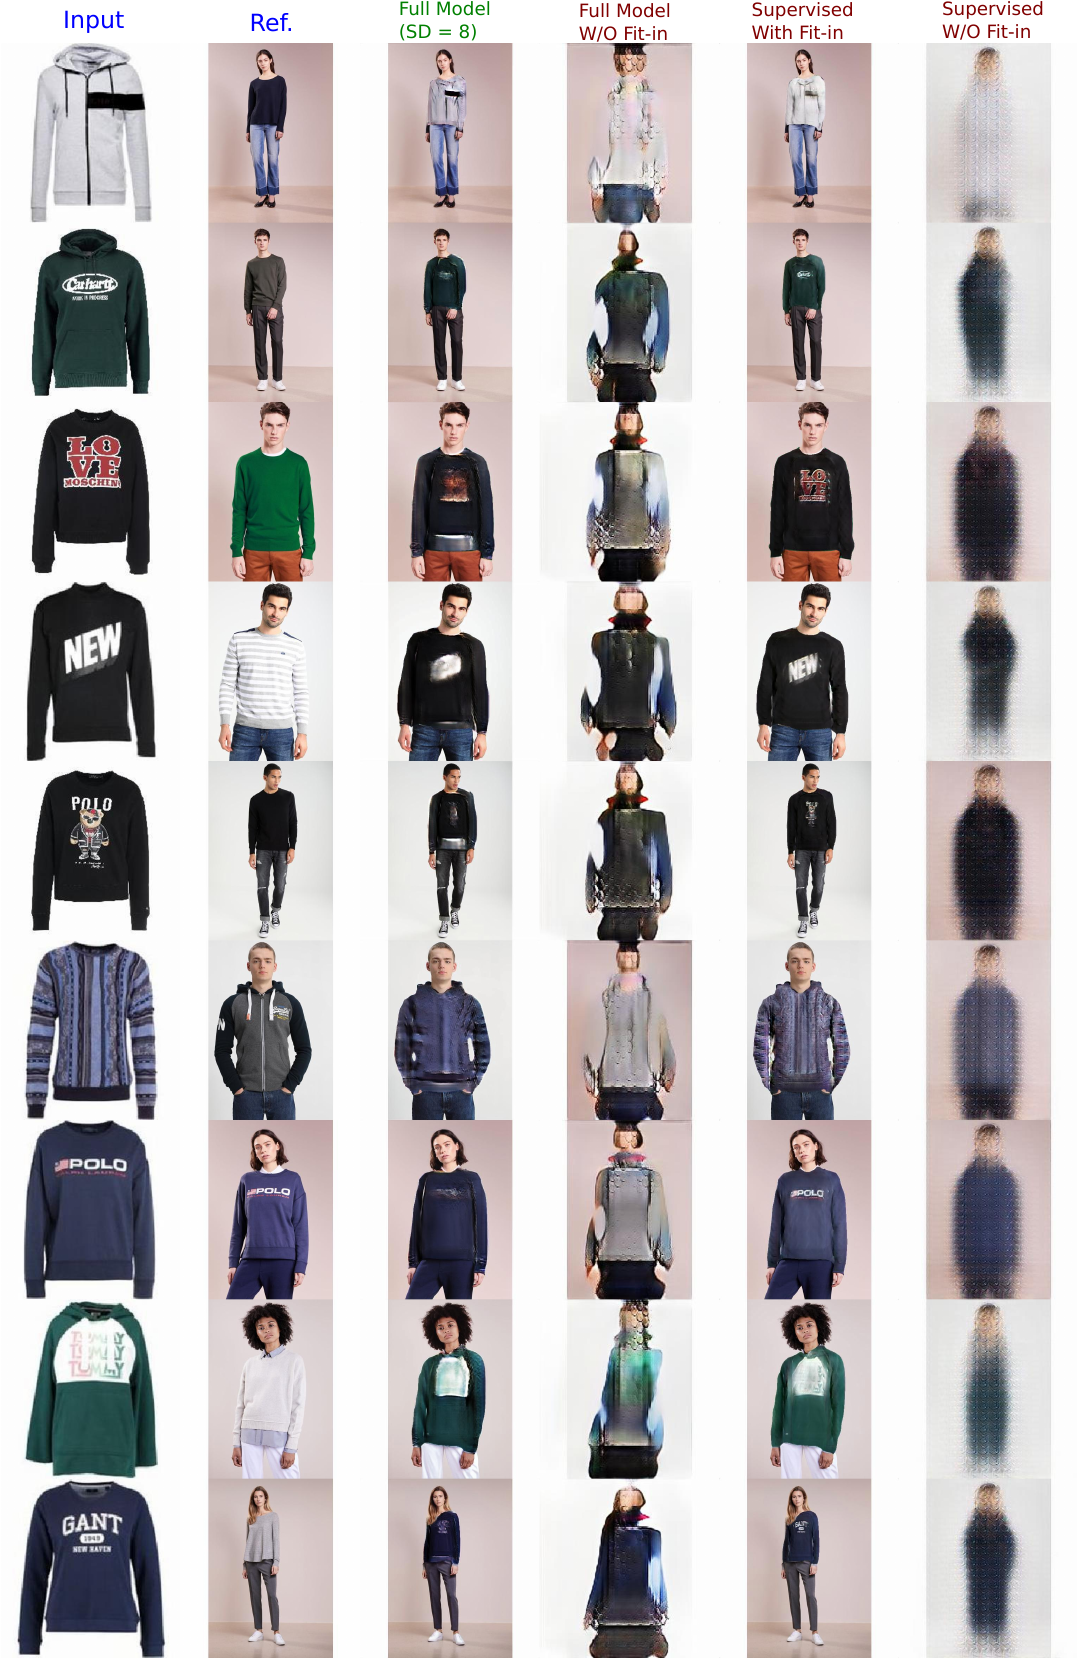}
\caption{
Comparison of our \textbf{unsupervised model}, \textbf{unsupervised model without Fit-in module}, \textbf{supervised model} and \textbf{supervised model
without using Fit-in module}.}
\label{fig:Supp_FashionStyle_super_fitin_p1}
% \vspace{-4mm}
\end{figure*}

\begin{figure*}[thb]
\centering
\includegraphics[width=0.8\textwidth]{supp_imgs/supp_spott_fitin_p2-crop.pdf}
\caption{
Comparison of our \textbf{unsupervised model}, \textbf{unsupervised model without Fit-in module}, \textbf{supervised model} and \textbf{supervised model
without Fit-in module}.}
\label{fig:Supp_FashionStyle_super_fitin_p2}
% \vspace{-4mm}
\end{figure*}

%%%%%%%%%%%%%%%%%%%%%%%%%%%%%%%%%%%%%%%%%%%%%%%%%%%%%
\begin{figure*}[thb]
\centering
\includegraphics[width=0.88\textwidth]{supp_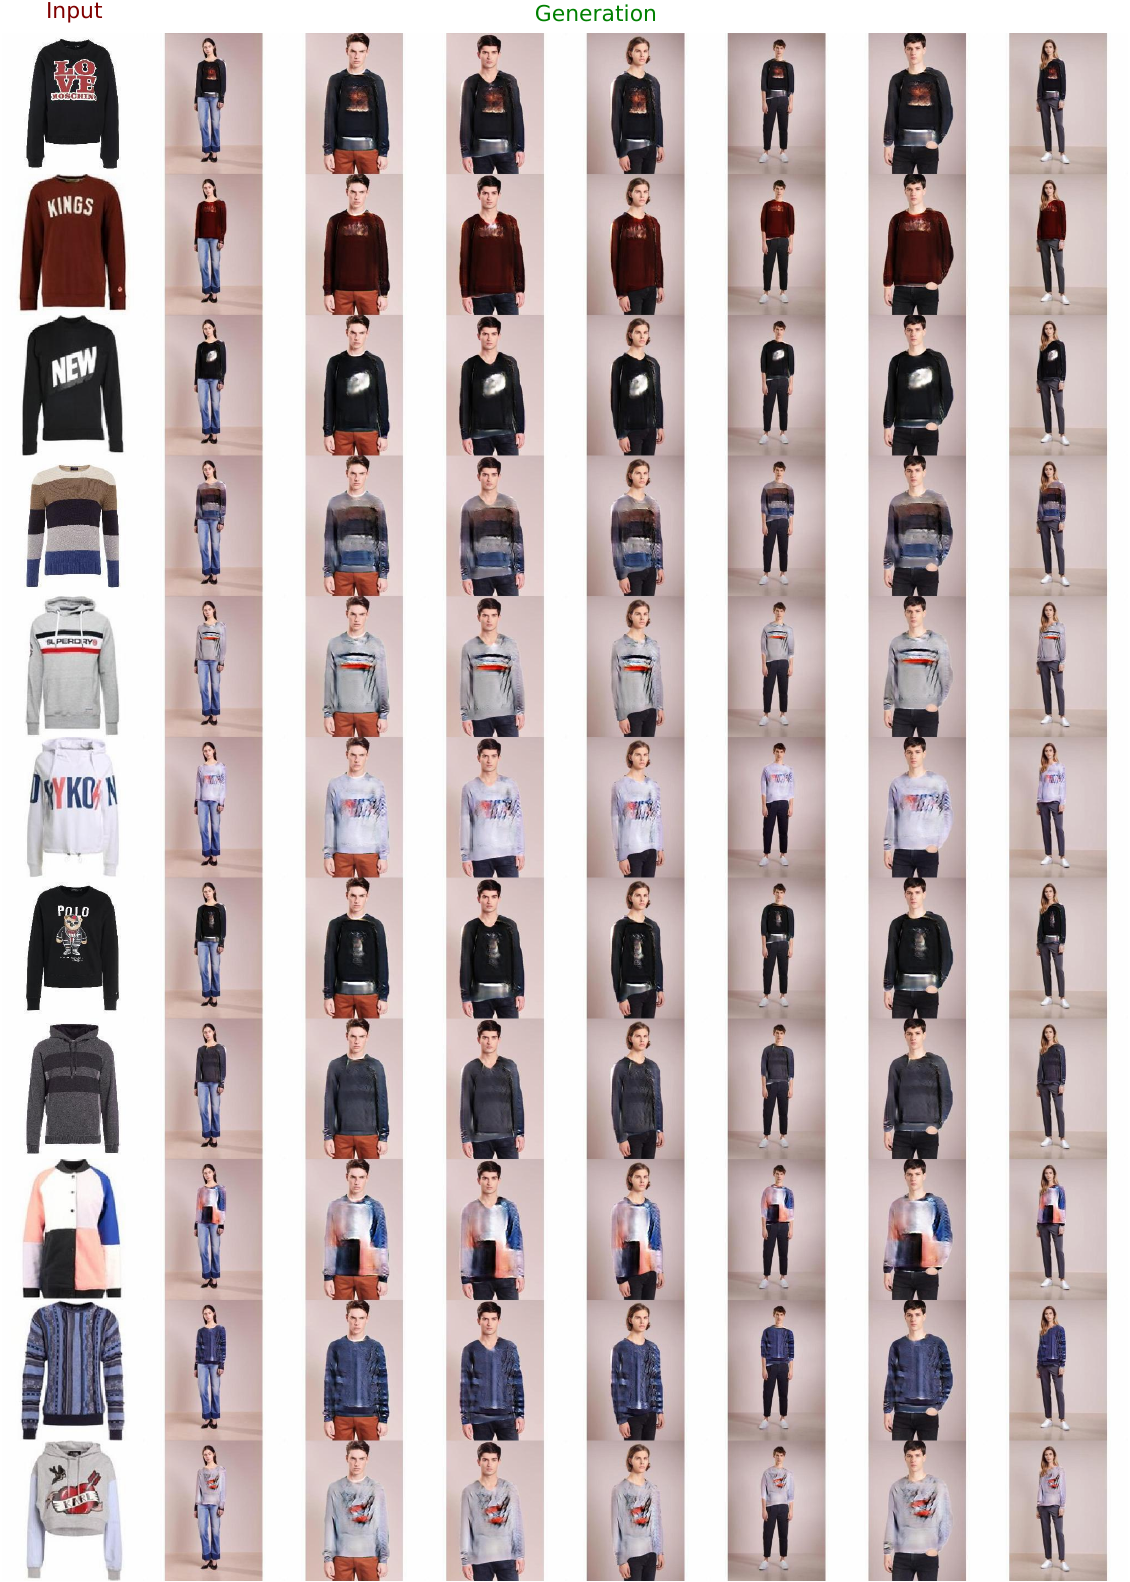}
\caption{
Qualitative results for the \textbf{Try-on} task on our FashionStyle dataset. The first column is the input clothing, the rests are virtual try-on results.}
\label{fig:Supp_FashionStyle_quality_tryon}
% \vspace{-4mm}
\end{figure*}

\begin{figure*}[thb]
\centering
\includegraphics[width=0.8\textwidth]{supp_imgs/supp_spott_quality_takeoff_v2-crop.pdf}
\caption{
Qualitative results for the \textbf{Take-off} task on our FashionStyle dataset. Each set contains three images: Input, generated take-off image and the reference ground truth.}
\label{fig:Supp_FashionStyle_quality_takeoff}
% \vspace{-4mm}
\end{figure*}

%%%%%%%%%%%%%%%%%%%%%%%%%%%%%%%%%%%%%%%%%%%%%%%%%%%%%
\begin{figure*}[thb]
\centering
\includegraphics[width=1\textwidth]{supp_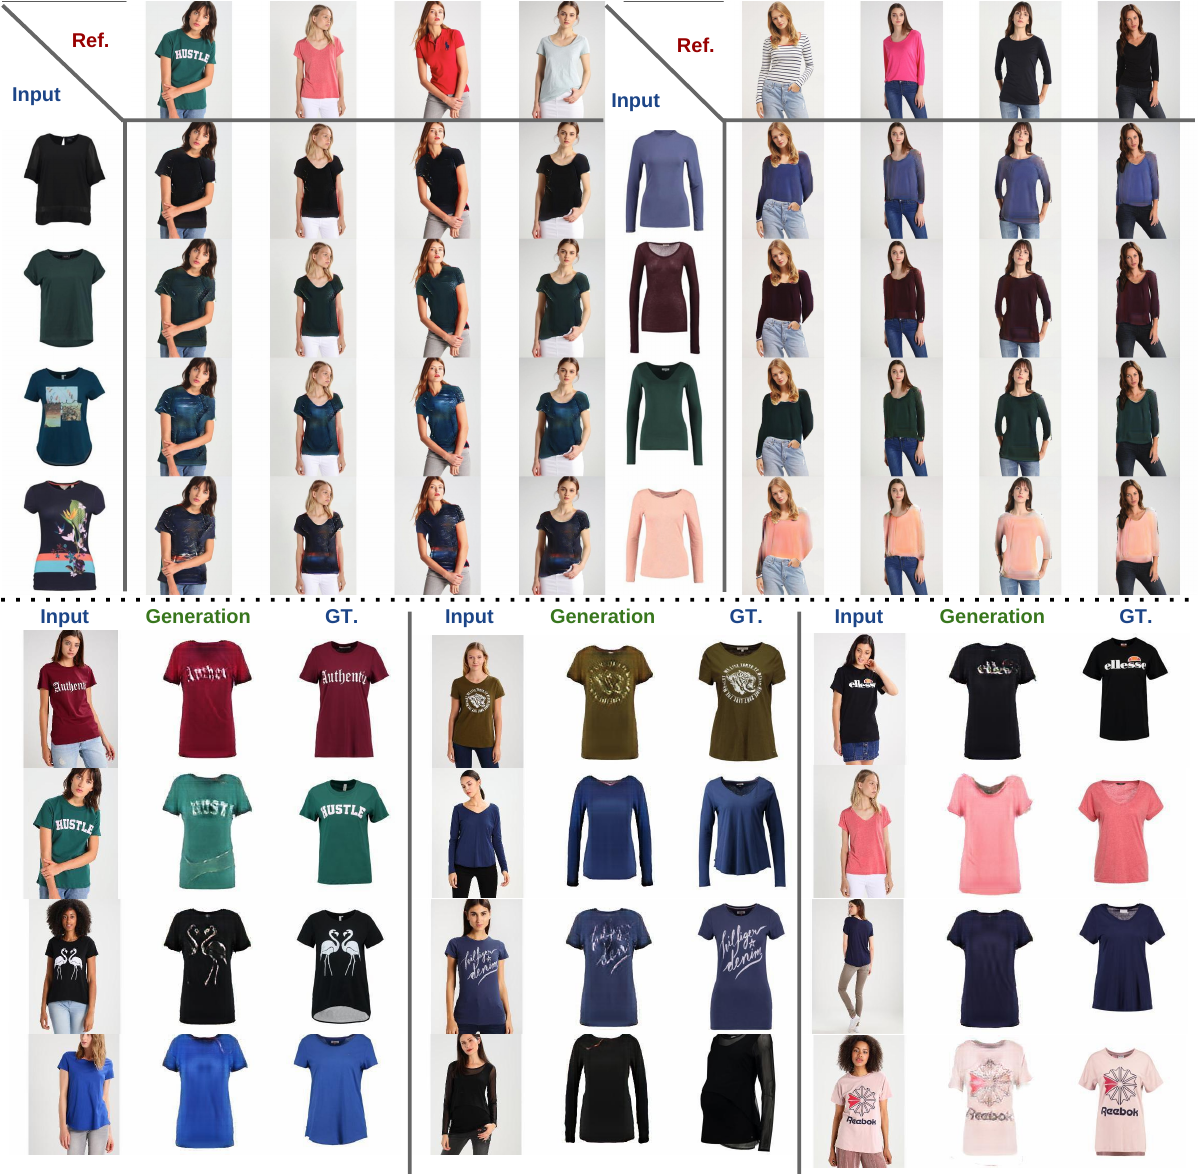}
\caption{
A larger size version of the qualitative results on the \textbf{VITON} dataset (related to Fig.~5 in the main paper).}
\label{fig:Supp_VITON_quality}
% \vspace{-4mm}
\end{figure*}

%%%%%%%%%%%%%%%%%%%%%%%%%%%%%%%%%%%%%%%%%%%%%%%%%%%%%
\begin{figure*}[thb]
\centering
\includegraphics[width=1\textwidth]{supp_imgs/retrieval_supp_v2-crop.pdf}
\caption{
More retrieval results on our FashionStyle dataset. Each three rows have two different query images but refer to the same product. }
\label{fig:Supp_retrieval}
% \vspace{-4mm}
\end{figure*}

%%%%%%%%%%%%%%%%%%%%%%%%%%%%%%%%%%%%%%%%%%%%%%%%%%%%%
\begin{figure*}[thb]
\centering
\includegraphics[width=0.85\textwidth]{supp_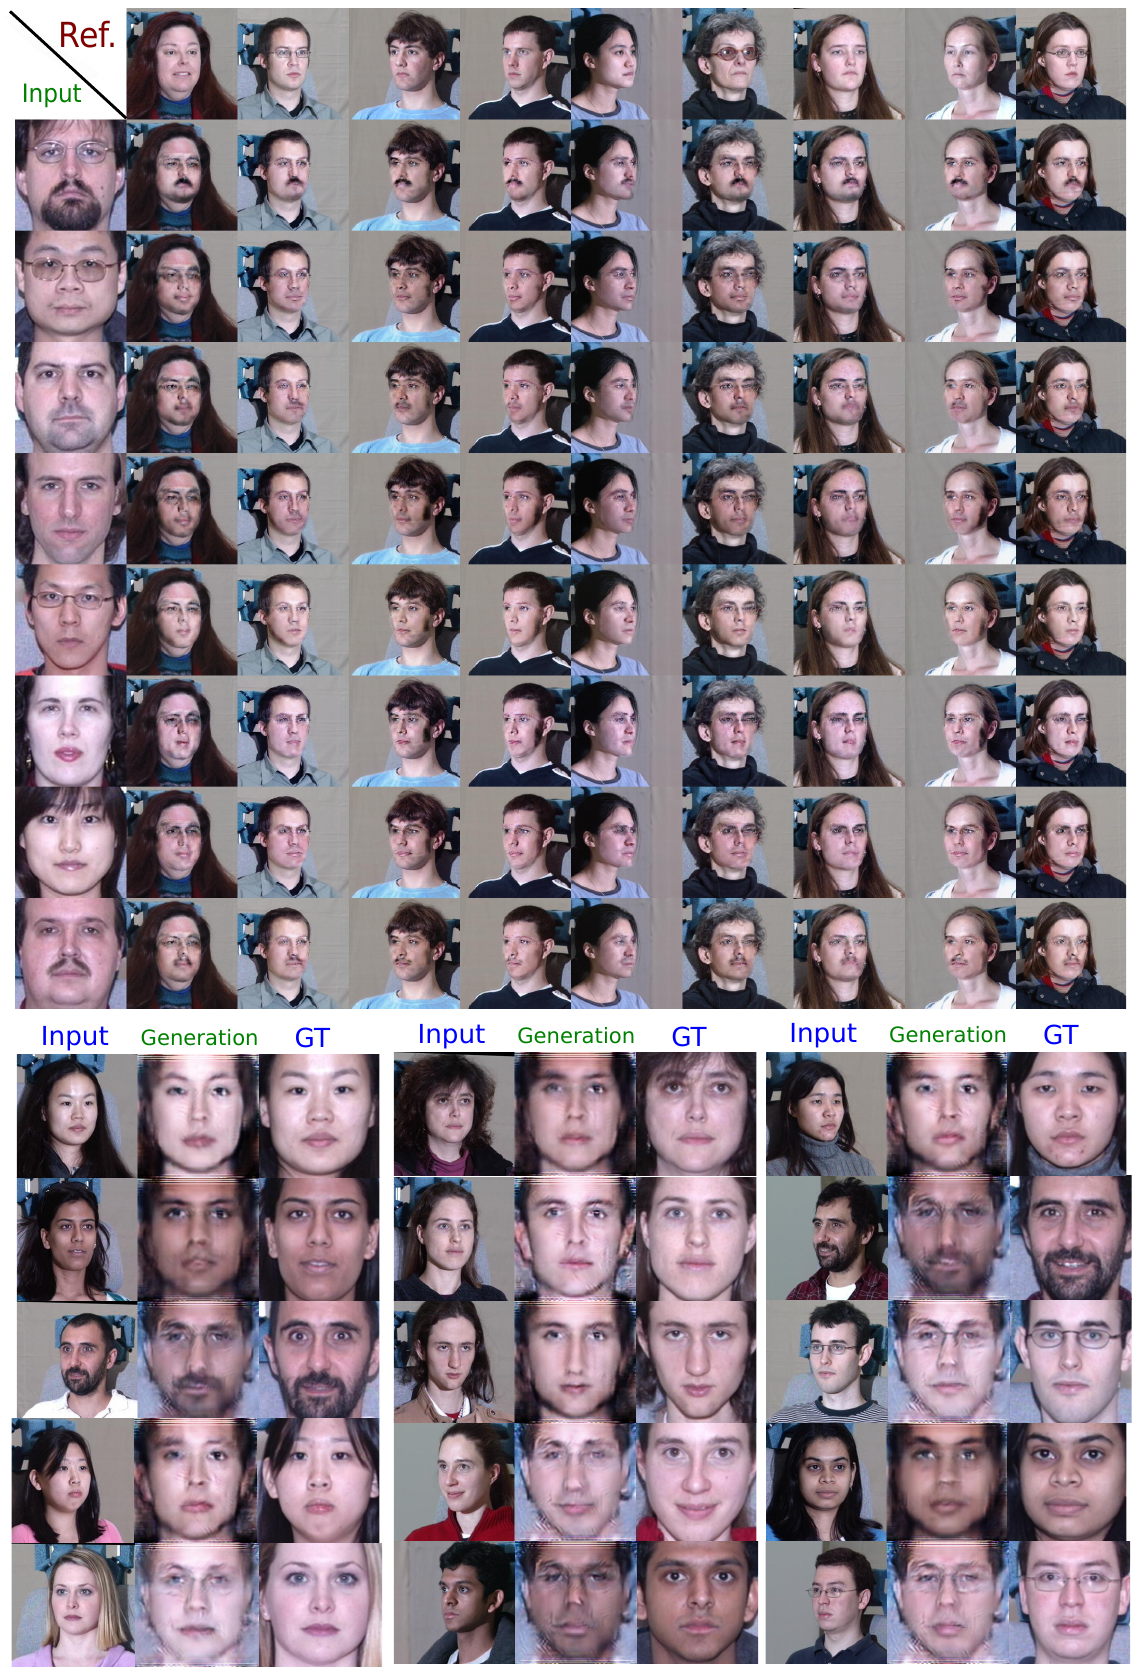}
\caption{
A higher resolution version of the qualitative results of the face translation (related to Fig.~9 in the main paper).}
\label{fig:Supp_face_quality}
% \vspace{-4mm}
\end{figure*}

\begin{figure*}[thb]
\centering
\includegraphics[width=0.9\textwidth]{latex/supp_imgs/tsne_ori-crop.pdf}
\caption{
t-SNE visualization of the testing images from Domain 2 by using the 8-dim style code. Please note the
blue circles are groups of stripe pattern.}
\label{fig:tsne_ori}
% \vspace{-4mm}
\end{figure*}

\begin{figure*}[thb]
\centering
\includegraphics[width=0.8\textwidth]{latex/supp_imgs/tsne_grid-crop.pdf}
\caption{
Grid version of t-SNE visualization of the testing images from Domain 2 by using the 8-dim style code.
Please note the blue circles are groups of stripe 
patterns, the red circle is a group of big logos.
}
\label{fig:tsne_grid}
% \vspace{-4mm}
\end{figure*}
%%------------------------------------------
% \vspace{-0.5cm}

%%===========================

\clearpage
\begin{table}[t]
\centering
% \footnotesize
% \begin{tabular*}{17cm}
\begin{tabular}
{@{\extracolsep{\fill}} l c c c c c c c c c c c c c}
\toprule 
Translation &$n_1$ &$n_2$ &$n_3$ & Minibatch & Learning rate & $\lambda_\text{CC}$ & $\lambda_\text{SR}$ & $\lambda_\text{LR}$ & $\lambda_\text{Sym}$ & $\lambda_\text{P}$ & $\lambda$ & Iteration  \\
\midrule[0.6pt]	
	Clothing try-on  &1 &3 &4 &1 &4e-5 &5 &10 &10 &10 & 5  &1e4 &$\sim$60k \\
	Clothing take-off &1 &3 &4 &1 &4e-5 &5 &10 &10 &10 & 2.5  &2e4 &$\sim$60k \\
	Face try-on &1 &2 &4 &2 &4e-5 &5 &10 &10 &10 &0.075 &6e5 &$\sim$60k \\
	Face take-off &1 &2 &4 &2 &4e-5 &5 &10 &10 &10 &0.025 &2e6 &$\sim$60k \\
\bottomrule[1pt]

\end{tabular}
\caption{Network architecture and training parameters details.}
% \vspace{+100mm}
\label{tab:param}
\end{table}
